# Supplementary material for: Learning from Rational Behavior: Predicting Solutions to Unknown Linear Programs
Source: arXiv:1506.02162 source file (2016-10-26)
Supplement: Supplementary file 1 [file updates-appendix.tex]

\section{Formal Description of the Update Rules in $\learnedge$}
\label{sec:appendix-updates}
We present the formal descriptions of the updates of $\learnedge$ in this section. Each update rule provide an update for only a portion
of the information $\cI\utt$\ifnum\final=0  at day $t$ given in \eqref{eq:info}.\else.\fi~For the items not mentioned in an update rule, we simply copy it over
into $\cI\uttf$.
%\rynote{Want to tie in the information $\cI$ into the update rules.   Want to word better.}
\begin{enumerate}[label=\textbf{U.\arabic*}]
%\item\label{u0}	Routine Update: $X\utt \gets X^{(t-1)} \cup \{\bbx\utt\}$ 
%\rynote{Got rid of the routine update in the update rules because it seemed nicer to break up the update rules into 4 mutually exclusive items.}

\item If \label{u1}$\bbx\utt \notin \tN\utt$, then set $\bbx^* \gets \bbx\utt$;

%\item\label{u2} Else if $\bbx\utt \notin \bar X\utt$ and there is no
%edge in $E\utt$ such that $\bbx\utt \in e$, then check if there
%exists a pair $\bbx,\bbx' \in X\utt$ such that
%$\{\bbx,\bbx',\bbx\utt \}$ are collinear. If so, add a new edge $e$
%to the learned edge set: $E\uttf \gets E\utt \cup \{ e\}$; \ar{Using
%$e$ in two different ways here. Haven't defined the use of $e$ when
%it is added as a new edge}

\item\label{u2} Else if $\bbx\utt\notin e$ for any $e\in E\utt$ and $\bbx\utt\notin X^{(t)}$, then update the edge set
$$E\uttf \gets E\utt \cup \coline(X^{(t)} , \bbx\utt).$$
%\rynote{Even if COLLINE gives $\emptyset$, we still update $E$ by this. }
% if $\coline(X^{(t-1)} , \bbx\utt) \neq \emptyset$;

\item\label{u3} Else if $\bbc\cdot \hat\bbx\utt > \bbc\cdot \bbx\utt$,
then there exists $\hat e \in E\utt$ such that $\hat\bbx\utt \in \hat
e$ and the algorithm updates the questionable interval along this
edge-space.  Let $(Q_{\hat e}^i)\utt$ be the questionable interval
containing $\hat\bbx\utt$. 
\begin{itemize}
\item If the length of $(Q_{\hat e}^i)\utt$
is less than $1/2^N$, update via $\elim((Q_{\hat e}^i)\utt, F_e\utt,
(Y_e^i)\utt)$. 
\item Otherwise,
\begin{equation}
(Q_{\hat e}^i)\uttf \gets  (Q_{\hat e}^i)\utt \backslash (Y_{\hat e}^i)\uttf \quad \text{ where } \quad (Y_{\hat e}^i)\uttf \gets \text{conv}\left( (Y_{\hat e}^i)\utt ,\hat\bbx\utt\right).
\label{eq:update_infeas}
\end{equation}
\end{itemize}
%% The algorithm then updates the midpoint $(M_e^i)\uttf$ to be the new
%% midpoint of $(Q_e^i)\uttf$.
%Further $Q_{\hat e}\uttf \gets (Q_{\hat e}^i)\uttf \cup (Q_{\hat e}^{i+1})\utt$ where the addition with $i$ is done mod $2$.

%\item \label{u4} Else if $\exists e' \in E\utt$ such that $\bbx\utt \in e'$ and $\bbc\cdot \hat\bbx\utt > \bbc\cdot \bbx\utt$ but our guess $\hat\bbx\utt \in C_{e}\utt$ is infeasible for some different $e \in E\utt$.  Similar to \ref{u2} we update the questionable region where $\hat\bbx\utt$ was in, that is if $\hat\bbx\utt \in (Q_e^i)\utt$ (for $i = 1$ or $2$) then we update $\hat\bbx\utt \in (Q_e^i)\uttf$ as in \eqref{eq:update_infeas}.

\item\label{u4} Else $\bbc\cdot \hat\bbx\utt < \bbc\cdot \bbx\utt$, then there exists $e \in E\utt$ such that $\bbx\utt \in e$ 
%but the algorithm's prediction $\hat\bbx\utt \in C\utt \cup \bar X\utt$ had a strictly smaller objective value.  Although from the condition $\bbc\cdot \hat\bbx\utt < \bbc\cdot \bbx\utt$ we cannot deduce anything about the feasibility of the algorithm's prediction on the edge we predicted on \ar{Don't know what ``on the edge we predicted on'' means here},
and the algorithm updates a questionable interval on the edge-space $e$.  Let $(Q_{e}^i)\utt$ be the questionable interval
containing $\bbx\utt$. 
\begin{itemize}
\item 
If the length of $(Q_{e}^i)\utt$ is less than $1/2^N$, update via $\elim((Q_{e}^i)\utt, F_e\utt, (Y_e^i)\utt)$.
\item Otherwise, %% If $\bbx\utt \in (Q_{e}^i)\utt$ (for $i = 0$ or $1$) then the algorithm updates this questionable region by setting:
%\sj{guess all the $\hat e$ are just copy-paste typos for $e$. changed them.}
\begin{equation}
(Q_{e}^i)\uttf \gets(Q_{e}^i)\utt \backslash (F_{e}^i)\uttf \quad \text{ where } \quad (F_{e}^i)\uttf \gets \text{conv}\left( F_{e}\utt, \bbx\utt \right).
\label{eq:update_feas}
\end{equation}
\end{itemize}
%\rynote{infeasible region is Y not I.  What do we update with $\elim$? Should be clear what output is here.}
%\sj{fixed!}
\end{enumerate}
%\snote{TODO: put down precision assumption on $\cP$; move the precision assumption in prelim to Known Constraints.}
\sj{spent like 5 minutes but still can't figure out where the extra comma before section 3.2 is coming from.}
\rynote{It was an apostrophe.  I got it!}
%%% END UPDATE RULES %%%%
